# Supplementary material for: Unifying Adversarial Training Algorithms with Flexible Deep Data Gradient Regularization
Source: arXiv:1601.07213 source file (2016-07-29)
Supplement: Supplementary file 1 [file appendix.tex]

\appendix

\subsection{DataGrad:  Approximate Deep Data Regularization}
\label{data_grad}
We present the \emph{DataGrad} algorithm for learning architectures that are robust to adversarials. The goal is to minimize loss with a $+\lambda R(\frac{\partial \loss}{\partial d[1]},\dots,\frac{\partial \loss}{\partial d[k]})$ regularizer (data gradient of the loss $\loss$).  To describe \emph{DataGrad} we will require the following notation:

\begin{enumerate}
\item $W_\ell$ is the weight matrix connecting layer $\ell-1$ to layer $\ell$ so that $W_\ell[j,i]$ is the weight on the edge from node $i$ in layer $\ell-1$ to node $j$ in layer $\ell$. Layer $0$ is the data layer. \textcolor{red}{Each row $j$ is the incoming weight vector to node $j$ of layer $\ell$}.
\item $f$ is an activation function, so $f(h_\ell)$ is applied to each element of $h_\ell$. 
\item $g$ is the derivative of the activation function. For example, if $f(z) = max(0,z)$ then $g(z)=0$ if $z\leq 0$ and 1 if $z>0$
\item $h_\ell$ is the vector of weighted inputs for layer $\ell$.  %$h^{\ell}_i = \sum\limits_{c\in\ch{n^\ell_i}} w^{\ell}_{ci}a^{\ell-1}_c$.
\item $a_\ell$ is the vector of activations for layer $\ell$. For layer $0$, $a_0$ is the data itself. Note that $a^{\ell}_i = f^\ell_i(h^\ell_i)$.
\item $\dout_\ell$ is the vector of derivatives of the $\textcolor{red}{loss}$ with respect to the $h$ values in layer $\ell$ (i.e. $h_\ell$).
\item $\circ$ is the Hadamard product
\item $\mathcal{R}$ is the regularizer that takes the data gradient (i.e. derivative of loss with respect to data, i.e. $\dout_0$) and returns a number (regularization penalty)
\item $\mathcal{S}$ is the gradient of the regularizer with respect to its input (a vector with the same dimension as the data): $[\frac{\partial R(\vec{x})}{\partial \vec{x}[1]}, \dots \frac{\partial R(\vec{x})}{\partial \vec{x}[n]}]$
\end{enumerate}

The regularizer term is $R(\frac{\partial \loss}{\partial d[1]},\dots,\frac{\partial \loss}{\partial d[k]})$ (where $k$ is the dimensionality of the data).
Then, letting $x$ be the data gradient,
\begin{align*}
\frac{dR}{dW_\ell[j,i]} &= \sum\limits_{r=1}^k \frac{\partial R(x)}{\partial x[r]}\frac{\partial^2\loss(W_\ell,d)}{\partial W_\ell[j,i]\partial d[r]}\\
&\approx \sum\limits_{r=1}^k \frac{\partial R(x)}{\partial x[r]}\frac{\partial^2\loss(W_\ell,d)}{\partial d[r]\partial W_\ell[j,i]}\quad\text{(equality at points of continuity)}\\
&= \frac{\partial}{t}\frac{\partial \loss(W_\ell, d+ty)}{\partial W_\ell[j,i]} \quad\text{(evaluated at $t=0$)}\\
%&\text{(where $y$ is the gradient of $R$ with respect to its inputs evaluated using the current data gradient)}
%&= \sum\limits_{r=1}^k \frac{\partial R(x)}{\partial x[r]}\frac{\partial}{\partial W_\ell[j,i]}\left(\frac{\partial\loss}{\partial d[r]}\right)\\
%&= \sum\limits_{r=1}^k \frac{\partial R(x)}{\partial x[r]}\frac{\partial}{\partial W_\ell[j,i]}\left(\sum_s \frac{\partial\loss}{\partial h_\ell[s]}\frac{\partial h_\ell[s]}{\partial d[r]}\right)\\
%&= \sum\limits_{r=1}^k \frac{\partial R(x)}{\partial x[r]}\frac{\partial}{\partial W_\ell[j,i]}\left(\frac{\partial\loss}{\partial h_\ell[j]}\frac{\partial h_\ell[j]}{\partial d[r]}\right)\quad\text{(only $h_\ell[j]$ is affected by $W_\ell[j,i]$}\\
%
%&\approx \sum\limits_{r=1}^k \frac{\partial R(x)}{\partial x[r]}\frac{\partial^2\loss}{\partial d[r]\partial W_\ell[j,i]}\\
%&=\sum\limits_{r=1}^k \frac{\partial R(x)}{\partial x[r]}\frac{\partial}{\partial d[r]}\left(\frac{\partial \loss}{\partial W_\ell[j,i]}\right)\\
%&=\sum\limits_{r=1}^k \frac{\partial R(x)}{\partial x[r]}\frac{\partial}{\partial d[r]}\left(\frac{\partial \loss}{\partial h_\ell[j]}\frac{\partial h_\ell[j]}{\partial W_\ell[j,i]}\right)\\
%&=\sum\limits_{r=1}^k \frac{\partial R(x)}{\partial x[r]}\frac{\partial}{\partial d[r]}\left(\frac{\partial \loss}{\partial h_\ell[j]}a_{\ell-1}[i]\right)\\
\end{align*}

\noindent
which is the deep Jacobian of the regularizer where $y$ is the gradient of $R$ with respect to its inputs evaluated using the current data gradient.

However, since the form of the data derivatives closely mirrors the form of the gradient with respect to the layer 1 weights, the computation of $\frac{\partial^2\loss(W_\ell,d)}{\partial W_\ell[j,i]\partial d[r]}$ would be similar to computing a large sub-block of the Hessian, which is slow \citep{bishophessian}. Instead, we notice we only need the value of this matrix times a vector, so we adapt the idea of Pearlmutter \citep{multiplyhessian} by using finite differencces as follows:

% Omitted "dgrad" since we don't actually use it in our Algorithm diagram?
\begin{itemize}
\item $\xi_\ell=$  the backprop gradient of $\loss(W_\ell,d)$ with respect to weights.
%\item $dgrad=$ the gradient of $\loss(W_\ell,d)$ with respect to the data.
\item $y=$ the gradient of $R$ with respect to its inputs, evaluated at $dout_0$.
\item $\omega_\ell =$ backprop gradient of  $\loss(W_\ell,d+ty)$ with respect to weights (i.e. add small adversarial noise to data and get backprop derivative for weights)
\item The gradient of the regularization term with respect to $W_\ell$ is $(\omega_\ell-\xi_\ell)/t$
\end{itemize}

Using the above finite-difference approximation of the deep Jacobian of the regularizer, \emph{DataGrad} requires four total passes through the neural architecture.  Explicitly, the steps are as follows: 1) compute layer-wise statistics (linear pre-activations, activations, etc.) and error derivatives $dout_{\ell}$ using a data sample $d$ (or mini-batch of such samples), 2) use the low-level error signal $dout_0$ calculate gradient $y$, 3) generate an adversarial sample via $\widehat{d} = d + t y$, and 4) compute layer-wise statistics and error derivatives $\widehat{dout}_\ell$ for the adversarial sample(s), and 5) calculate parameter gradients and the approximate deep Jacobian of the regularizer and update model parameters via gradient descent.  The full \emph{DataGrad} procedure is detailed in Algorithm \ref{algo:ddgb2}.

\begin{algorithm}
\DontPrintSemicolon 
\KwIn{One data record $d=(d_1,d_2,\dots)$}
\KwIn{Learning Rate $\eta$, regularization meta-parameter $\lambda$}
\KwOut{Updates the weights}
\tcp*[l]{\red{Forward Phase I (Feed Forward)}}
\For{Layer $\ell\gets 1$ \textbf{to} $K$}{
        $h_\ell \gets W_\ell a_{\ell-1}$\;
        $a_\ell \gets f(h_\ell)$\;
}
prediction$\gets a_K$\;
loss$\gets\loss(t,a_K)$\;
\tcp*[l]{\red{Backward Phase (gather backprop information, don't update yet)}}
lossderiv$\gets$ gradient of loss  $\loss(t,a_K)$ with respect to the second parameter (predictions)\;
\tcp*[l]{Top layer first}
$\dout_K \gets g(h_K)\hadamard $ lossderiv \tcp*{$\partial$ loss / $\partial h_K$ }
\tcp*[l]{Middle layers and bottom layer}
\For{Layer $\ell \gets K-1$ to $1$}{
    $\dout_\ell\gets (W_{\ell+1}^T\dout_{\ell+1})\hadamard g(h_\ell)$\tcp*{$\partial$ loss / $\partial h_\ell$ }
}
\tcp*[l]{Data gradient from data layer}
$\dout_0\gets W_1^T \dout_1$\;
\tcp*[l]{\red{Finite differencce update phase}}
\tcp*[l]{new image obtained by adding small multiple of data gradient to image}
$y\gets$ gradient of $\mathcal{R}$ with respect to its immediate input, evaluated at $\dout_0$\;
$\widehat{d} \gets d + ty$ \tcp*{for some small $t$, $\hat{d}$ is an adversarial}
Repeat Steps 1-9 for $\widehat{d}$ to obtain appropriate $\widehat{a}_{\ell}$ and $\widehat{\dout}_\ell$ back-prop statistics\;
\For{$\ell=1$ to $K$}{
backproptmp$_\ell$ $\gets \dout_\ell * a_{\ell-1}^T$\tcp*{a matrix, derivative of loss with respect to weights}
secondbackproptmp$_\ell$ $\gets \widehat{\dout}_\ell * \widehat{a}_{\ell-1}^T$ backprop derivatives for layer $\ell$ at same weights but new image $\widehat{d}$.\;
$\text{regrad}_\ell \gets$ (secondbackproptmp$_\ell$ - backproptmp$_\ell$)$/t$\;
$W_\ell\gets W_\ell - \eta(\text{backproptmp}_\ell + \lambda*\text{regrad}_\ell)$\;
}

\caption{Deep data-gradient backprop in matrix form (regularization is on gradient of loss with respect to data)}
\label{algo:ddgb2}
\end{algorithm}

%\begin{figure}
%\includegraphics[width=\linewidth]{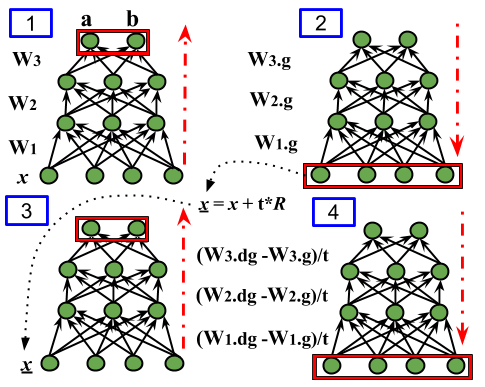}
%\caption{The flow process of the DataGrad regularizer.}
%\end{figure}
